# Supplementary material for: Resolving Dynamic Properties of Polymers through Coarse-Grained Computational Studies
Source: arXiv:1601.03289 source file (2016-01-13)
Supplement: Supplementary file 1 [file prl_2015_salerno_supp.pdf]

Supplemental Information

# Resolving Dynamic Properties of Polymers through Coarse-Grained Computational Studies

K. Michael Salerno,[1] Anupriya Agrawal,[2,3] Dvora Perahia,[2] and Gary S. Grest[1]

[1]Sandia National Laboratories, Albuquerque, NM, 87185

[2]Department of Mechanical Engineering and Materials Science, Washington University, St. Louis, MO 63130

[3]Department of Chemistry, Clemson University, Clemson, SC 29634

For our atomistic melt simulation 2800 polyethylene chains of length n = 96 were equilibrated for 30 ns at 500K and density 0.72 g/cm$^3$. Over this equilibration chains move a distance equivalent to their end-to-end distance $<R^2>$, indicating that no memory of the initial state remains. The simulations were run in the NVE ensemble with a Langevin thermostat with damping time constant 1 ps and time step $\delta t = 4$ fs. The RESPA multistep integrator [1] was used to integrate bond, angle, dihedral and non-bonded interactions with a 1 fs time step and to integrate the long-range electrostatics with a 4 fs time step. Atomistic particle configurations were sampled every 0.1 ns over 7 ns. Over this time the chains move a significant distance relative to their end-to-end size, indicating that many local conformations are sampled during this interval. Samples were used to generate the bond and angle distributions shown in Fig. S1 and nonbonded radial distribution functions g(r) shown in Fig. S2. In addition to this n = 96 sample, a system of 216 chains of length n = 480 polymer chains were also simulated. Both the n = 96 and 480 systems were used to calibrate the time scaling for each of the CG potentials.

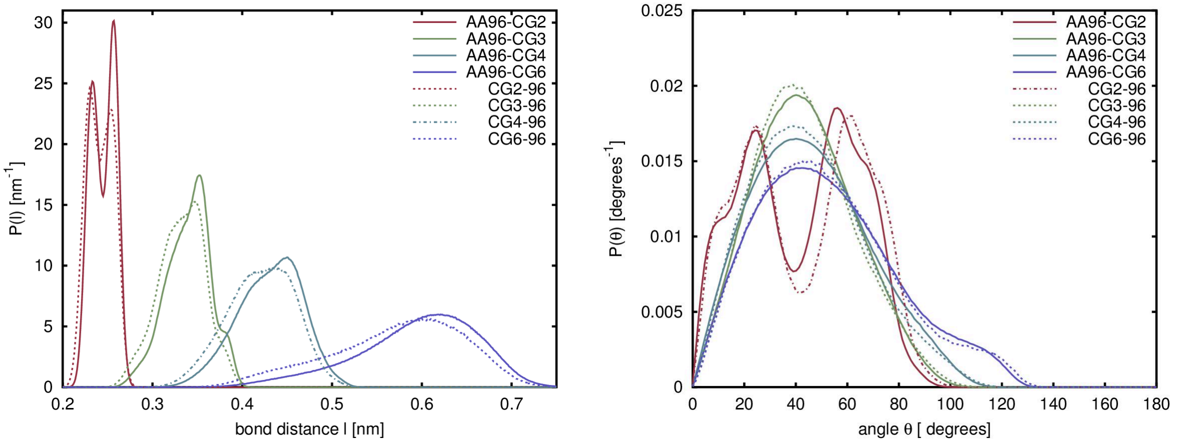


Figure S1 Bond length and angle distributions for each of the CG models (dashed) as well as the target distributions from the n=96 atomistic simulations (solid).

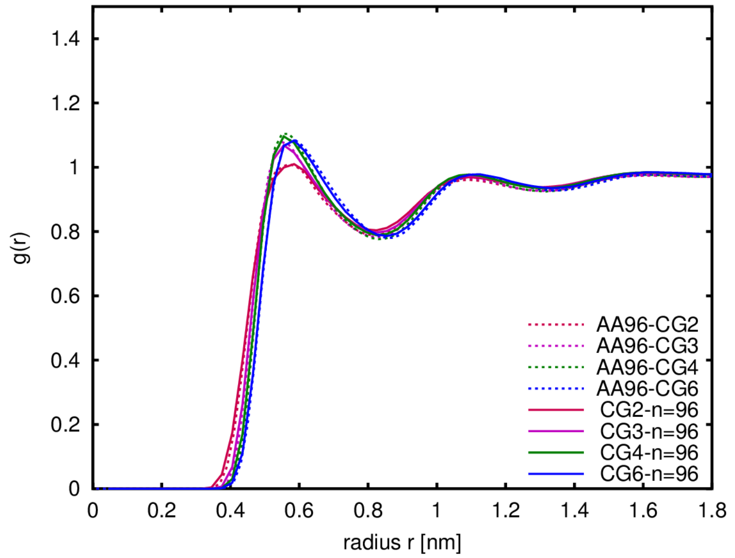


Figure S2: The target intermolecular radial distribution function g(r) for each coarse-grained model from the atomistic n=96 sample (solid) as well as the final distribution from the CG simulations (dashed).

For the atomistic simulations, the attractive $r^{-6}$ dispersion term in the Lennard-Jones interaction and the electrostatic interactions were calculated using particle–particle particle mesh algorithm [2]. Interactions closer than 1.2 nm are calculated in real space; those outside this range are calculated in reciprocal Fourier space with precision of 3 x $10^{-5}$. The repulsive $r^{-12}$ Lennard-Jones interaction is truncated at 1.2 nm. For the CG models the nonbonded interaction was truncated at 1.0 nm. All simulations in this paper were performed using the parallel molecular dynamics code Large Atomic Molecular Massive Parallel Simulator (LAMMPS) [3].

For each of the CG models 345 chain n = 96 and 316 chain n = 480 samples were initially simulated in the NPT ensemble with a target pressure P = 30 atm to calculate the density for each model. Samples at these densities were simulated in long production runs in the NVE ensemble. For the n = 960 and n = 1920 chain lengths a constant density ρ = 0.762 g/cm$^3$ was used for all of the CG models. These simulations contained 216, 800 and 800 chains respectively. The density was determined from NPT simulations of CG3 and CG4 model n = 960 chains at 30 atm. Without the non-crossing constraint the CG6 model also matched this density.

All simulations of CG models utilized a Langevin thermostat with damping time constant 20 ps. To determine the time step δt for the CG models, we ran a series of simulations with different time steps for each λ for n = 96. The largest time step that in conjunction with the Langevin damping constant kept temperature stable for a million steps was used in the simulations.

For the CG6 model the modified segmental repulsive potential developed by Sirk et al was applied [4]. A bond bead diameter of 0.5 nm was chosen to prevent chain crossing. For smaller bead sizes chain crossing occurred, resulting in a chain-length dependent scaling factor α. We observed no significant change in g(r) in simulations using the 0.5 nm bead diameter. A comparison of g(r) for a CG6 model that uses the non-crossing constraint and for a CG6 model that does not is shown in Fig. S3, with only minor differences observed.

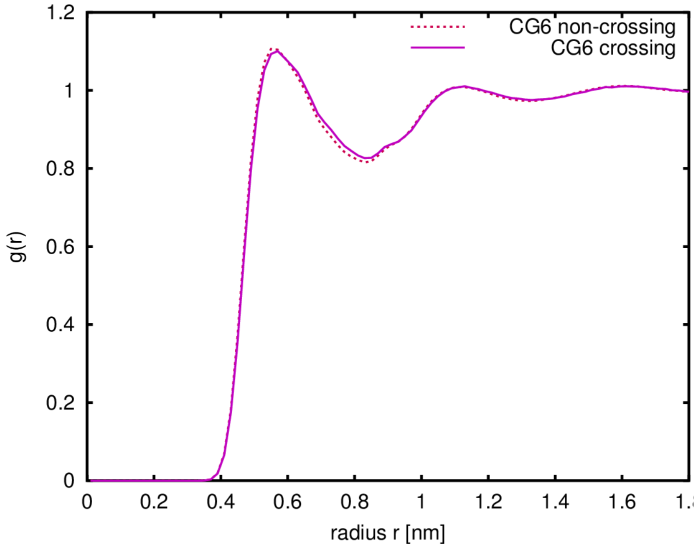


Figure S3: The intermolecular radial distribution function g(r) for the CG6 model with the non-crossing constraint applied (dashed) without the non-crossing constraint (solid).

Three factors contribute to the speedup in a CG model, the time scaling factor α, the time step δt, and the reduction in the number of degrees of freedom relative to the atomistic model. The reduction of the number of degrees of freedom represents the number of atoms combined into each CG bead or 3λ for a CGλ model of polyethylene. These three quantities are listed for each of the models in Supplemental Table 2. The theoretical speedup relative to the atomistic model is $\alpha \times \delta t \times (3\lambda)^2$, which for the CG4 model yields a theoretical speedup of about 20,000 relative to the atomistic simulation. The realized speedup of the CG4 model is nearly 30,000, due in part to a smaller cutoff in the CG simulations.

Supplementary Table 1

| $C_nH_{2n+2}$ | CG Model | $\langle R^2 \rangle$ [$nm^2$] | Density [$g/cm^3$] |
|---|---|---|---|
| 96 | AA | 14.56 | 0.72 |
| | CG2 | 12.73 | 0.72 |
| | CG3 | 16.85 | 0.73 |
| | CG4 | 17.74 | 0.73 |
| | CG4M | 22.21 | 0.73 |
| | CG6 | 15.42 | 0.72 |
| | UA | 12.02 | 0.80 |
| 480 | AA | 88.64 | 0.73 |
| | CG2 | 68.78 | 0.76 |
| | CG3 | 94.41 | 0.76 |
| | CG4 | 101.13 | 0.76 |
| | CG4M | 124.74 | 0.76 |
| | CG6 | 88.27 | 0.76 |
| | UA | 66.41 | 0.81 |
| 960 | CG2 | 136.17 | 0.76 |
| | CG3 | 194.16 | 0.76 |
| | CG4 | 205.72 | 0.76 |

| | | | |
|---|---|---|---|
| | CG4M | 255.20 | 0.76 |
| | CG6 | 181.15 | 0.76 |
| 1920 | CG3 | 376.72 | 0.76 |
| | CG4 | 382.35 | 0.76 |
| | CG4M | 482.39 | 0.76 |
| | CG6 | 365.25 | 0.76 |

Supplementary Table 2

| Model | Time scaling α | Timestep δt | 3λ |
|---|---|---|---|
| Atomistic | 1 | 1 fs | - |
| UA | 1.4 | 2 fs | 3 |
| CG2 | 8.2 | 2 fs | 6 |
| CG3 | 7.4 | 10 fs | 9 |
| CG4 | 6.9 | 20 fs | 12 |
| CG4-M | 2.2 | 20 fs | 12 |
| CG6* | 9.5 | 20 fs | 18 |

* without the non-crossing constraint, which reduces the effective value of 3λ

## References


[1] M. Tuckerman, B. J. Berne, and G. J. Martyna, J. Chem. Phys. 97, 1990 (1992)

[2] R. Isele-Holder, W. Mitchell, and A. E. Ismail, J. Chem. Phys. 137, 174107 (2012)

[3] S. Plimpton, J. Comput. Phys. 117, 1 (1995)

[4] T. W. Sirk, Y. R. Slizoberg, J. K. Brennan, M. Lisal, and J. W. Andzelm, J. Chem. Phys 136, 134903 (2012)
